# Supplementary material for: Intensity-Correlation Synthetic Wavelength Imaging in Dynamic Scattering Media
Source: arXiv:2510.27620 ancillary file (2025-10-31)
Supplement: Supplementary file 1 [file SupplementaryMaterial_Kassem_Intensity_Correlation_SWI.pdf]

# Supplementary Material: Intensity-Correlation Synthetic Wavelength Imaging in Dynamic Scattering Media

## S1. RECONSTRUCTION OPTIMIZATION ALGORITHM.

If an initial optical field $E_0(x, y, 0)$ is propagated by a distance $z$, then the optical field $E(x, y, z)$ in a plane at a distance $z$ can be written using the angular spectrum approach as [S1]:

$$E(x,y,z) = \int\int df_x df_y [\hat{E}(f_x, f_y, 0) exp(iz\alpha)] exp[i2\pi(f_x x + f_y y)] \tag{S1}$$

Here, $\hat{E}(f_x, f_y, 0)$ is the Fourier transform of the source optical field $E_0(x, y, 0)$. $f_x$ and $f_y$ are the spatial frequencies corresponding to the $x$ and $y$ axes and $\alpha$ is given by:

$$\alpha = \sqrt{\left(\frac{2\pi}{\lambda}\right)^2 - 4\pi^2(f_x^2 + f_y^2)} \tag{S2}$$

The optical field evolution represented in Eq. (S1) can be seen as the output of three mathematical operations acting on the source field: A Fourier transform operation represented by $\hat{FT}$ that takes as its input the source field and performs the 2-D Fourier transform. This is followed by multiplication operation by the transfer function i.e. $exp(iz\alpha)$ represented by $\hat{H}$ and finally the inverse Fourier transformation represented by $I\hat{FT}$.
For our experimental conditions, as a first approximation, we assume free space propagation through the medium because the synthetic wavelengths are in the $mm$ range. In this approximation, the measured/computed optical field $E_m$ via the $g^{(2)}$ correlations can be modelled as the propagated field of the object plane field $E(x, y, 0)$ in line with the angular spectrum model. In matrix operator notation, the measured field $E_m$ can then be represented as:

$$E_m = I\hat{FT}[\hat{H}[\hat{FT}E(x,y,0)]] + \epsilon = \hat{A}E + \epsilon \tag{S3}$$

Here, $\epsilon$ represents the noise registered in the measurement. The problem of retrieving the field $E(x, y, 0)$ can be modelled as that of a minimisation of a cost function $C(\widetilde{E})$ given by:

$$C(\widetilde{E}) = \frac{1}{2}||\hat{A}\widetilde{E} - E_m||^2 + \alpha TV(\widetilde{E}, \widetilde{E}^*) \tag{S4}$$

The first term is the data fidelity term that enforces the similarity with the measurements. The second term has the isotropic TV function weighted by a constant $\alpha$ and is defined as [S2] :

$$TV(\widetilde{E}, \widetilde{E}^*) = ||\nabla\widetilde{E}||_1 = \sum_i \sqrt{(\nabla_x\widetilde{E}_i)(\nabla_x\widetilde{E}_i^*) + (\nabla_y\widetilde{E}_i)(\nabla_y\widetilde{E}_i^*)} \tag{S5}$$

The iterative solution to the problem using the gradient descent proceeds by making an updated guess in each iteration as follows:

$$\widetilde{E}_i^{(n+1)} = \widetilde{E}_i^{(n)} - t[\nabla_{\widetilde{E}_i^*} C(\widetilde{E}_i, \widetilde{E}_i^*)]_{\widetilde{E}_i = \widetilde{E}_i^{(n)}} \tag{S6}$$

The functional gradient for the cost function is given by [S2] :

$$\nabla_{\widetilde{E}_i} C(\widetilde{E}_i) = \hat{A}^\dagger(\hat{A}\widetilde{E} - E_m) - \alpha\nabla.\left(\frac{\nabla\widetilde{E}_i}{|\nabla\widetilde{E}_i|}\right) \tag{S7}$$

Here, the gradient has to be taken with respect to the conjugate of the decision variable. $\hat{A}^\dagger$ represents the adjoint of the operator $\hat{A}$ defined in Eq. (S3) and can be written explicitly as:

$$\hat{A}^\dagger = \{I\hat{FT}\hat{H}\hat{FT}\}^\dagger = \{\hat{FT}^\dagger\hat{H}^\dagger I\hat{FT}^\dagger\} = \{I\hat{FT}\hat{H}^*\hat{FT}\} \tag{S8}$$

For reconstructing the object hidden behind volume scatterers we employ the measurements made with the multiple synthetic wavelengths. In that case the cost function to be minimized becomes the following:

$$C(\widetilde{E}) = \sum_{n=1}^{N} \frac{1}{2}||\hat{A}_{\lambda_n}\widetilde{E} - E_{m_n}||^2 + \alpha TV(\widetilde{E}, \widetilde{E}^*) \tag{S9}$$

Here, $\lambda_n$ represents the synthetic wavelengths for the $N$ measurements. The operator $\hat{A}$ represents the synthetic wavelength values that enter the transfer function operator $\hat{H}$ through $\alpha$ in Eq.S2. Therefore, the first term represents the data fidelity term for the measurements $E_{mn}$ corresponding to the different synthetic wavelengths.

## S2. SCATTERERS AND SCATTERING STRENGTHS.

For the two-plane scattering experiments, we used two N-BK7 ground glass diffusers (120-grit and 220-grit) of size 100 × 100 mm from Thorlabs. These diffusers have an average surface roughness ($\sigma_h$) of approximately 120-grit ($\sigma_h = 5.7\,\mu$m) and 220-grit ($\sigma_h = 3.5\,\mu$m) [S3].

The optical path length variations introduced by the diffusers are given by [S4]:

$$\Psi = 2\sigma_h \tag{S10}$$

Using the Rayleigh criterion in Eq. 13 of the main text, we determine that the wavelength $\Lambda$ should be larger than 45.6 $\mu$m and 28 $\mu$m. This means that, while optical waves (850 nm) would be highly scattered, the synthetic wavelength passes through it without any issues. For the actual two-scattering-plane setup, the effective $\Psi$ is much larger and scales with the geometry, including the distance between the two scattering planes, numerical aperture (NA), and other factors.

For the volume scattering experiment, we molded epoxy resin with $TiO_2$ particles to create volume scatterers of approximately 5.5 × 8 mm in $x$-$y$ dimension with different thicknesses. The total optical path length variations are given by [S4]:

$$\Psi = 2\frac{L^2}{l^*} = 2L^2\mu^* \tag{S11}$$

The scattering parameters and optical path lengths $\Psi$ changes of the samples are as follows:

| Sample | $\mu_s'$ (mm$^{-1}$) | Thickness (mm) | $\Psi$ (mm) | $\Lambda_{min}$ (mm) |
|---|---|---|---|---|
| A | 0.22 | 2.7 | 3.2 | 12.8 |
| B | 1.1 | 0.7 | 1.1 | 4.4 |
| C | 1.1 | 1.5 | 5.0 | 20 |

TABLE I. Optical parameters and total path length variations of the volume scatterers.

Here, we see that we are not fulfilling the Rayleigh criterion in Eq.13 (of the main text), as evidenced by the reconstructions in Fig.3 (of the main text), which show a significant amount of speckle. However, increasing the synthetic wavelength (SWL) would result in lower resolution. Therefore, we worked in this lightly scattering regime and applied denoising and spectral fusion techniques to address the issue.

## S3. DIFFRACTION LIMITED RESOLUTION

The theoretical resolution limit of our system is according to Abbe diffraction limit:

$$\delta_x = \frac{\Lambda}{2\ \mathrm{NA}} \tag{S12}$$

The numerical aperture (NA) is defined as,

$$NA = n\sin(\alpha_G) \approx n\tan(\alpha_G) = \frac{D}{\mathrm{z}} \tag{S13}$$

The approximation $\sin(\alpha) \approx \tan(\alpha)$ is valid for small numerical apertures (NA), but becomes inaccurate for large NAs. Therefore, we obtain:

$$NA = \frac{r}{\sqrt{r^2 + (\mathrm{z})^2}} \tag{S14}$$

The diffuser will function as an entrance pupil, thereby limiting the possible values of $k_x$ and $k_y$ and subsequently the NA. This will give a resulting resolution as a term of our experimental setup:

$$\delta_x = \frac{\Lambda\sqrt{r^2 + (\mathrm{r})^2}}{2r} \tag{S15}$$

Therefore, ideally, the final reconstruction resolution is determined by the synthetic wavelength and the distance between the diffuser and the object.

In the experiment, we used a fiber tip as a point source to demonstrate this theoretical limit. However, the fiber is not a true point source, as it has a finite divergence angle upon exiting the tip. At short distances from the scattering plane (as shown in Fig. S1), the NA of the fiber itself limits the total system's NA, resulting in a deviation from the Abbe limit and a plateau in the achievable resolution, as seen in Fig.4 of the main text, for short distances.

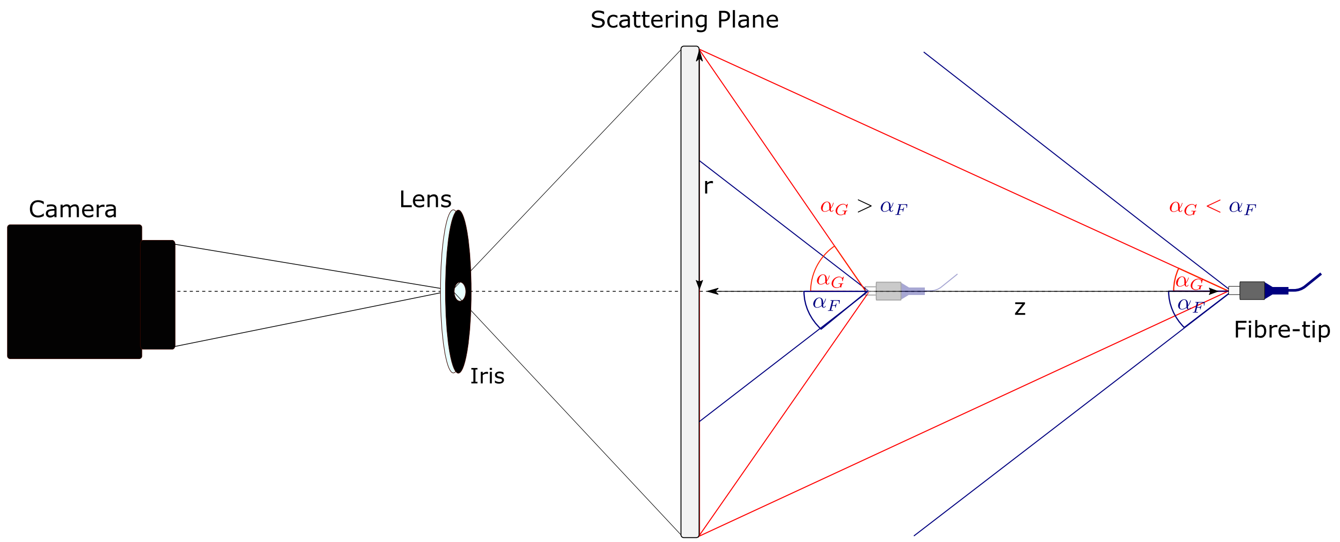


FIG. S1. Experimental setup for measuring the diffraction limit. A fiber tip, acting as a point source at the synthetic wavelength, is placed at varying distances to verify its adherence to the Abbe limit. While ideally a point source, the fiber has a finite divergence angle $\alpha_F$, which can be smaller than the geometric angle $\alpha_G$ at short distances.

## S4. ACQUISITION SPEED

An important consideration is the total acquisition time, which depends on the specific problem we aim to address.

To evaluate this, we used all of the collected frames (1000) to reconstruct the object and establish a ground truth (GT). We then progressively reduced the number of frames and computed the structural similarity index measure (SSIM) between the new reconstruction and the GT. The results are shown in Fig. S2.

We found that, in all cases, 200 frames are sufficient to achieve a reasonable reconstruction. For simpler problems, such as imaging through two diffusers in transmission, this can be further reduced to 50 frames.

## S5. DERIVATION OF THE EQUATIONS FOR $g^{(2)}$ MEASUREMENTS.

In the context of analysing second-order interferometric correlations, the Mach-Zehnder interferometer serves as a starting point. Here, an incoming electric field $\mathbf{E}$ is split into two distinct paths, producing the electric fields $E_1$ and $E_2$. These fields then recombine at a beamsplitter, creating a sum of fields measured at the output of the interferometer. For simplification, we assume identical electric field amplitudes and co-located fields in space, allowing us to treat the problem in only the time and frequency domains. The electric fields at the output ports, labelled $E_A$ and $E_B$, can be expressed as:

$$\begin{aligned} E_A(t_1, t_2, t) &= \frac{1}{\sqrt{2}} \left[ E_1(t - t_1) + jE_2(t - t_2) \right], \\ E_B(t_1, t_2, t) &= \frac{1}{\sqrt{2}} \left[ E_2(t - t_2) + jE_1(t - t_1) \right], \end{aligned} \tag{S16}$$

where $t$ is the global time, and $t_i$ represents the time taken by the electric field to traverse path $i$ in the interferometer. Assuming plane waves for the electric fields in both paths, we can express the individual fields as:

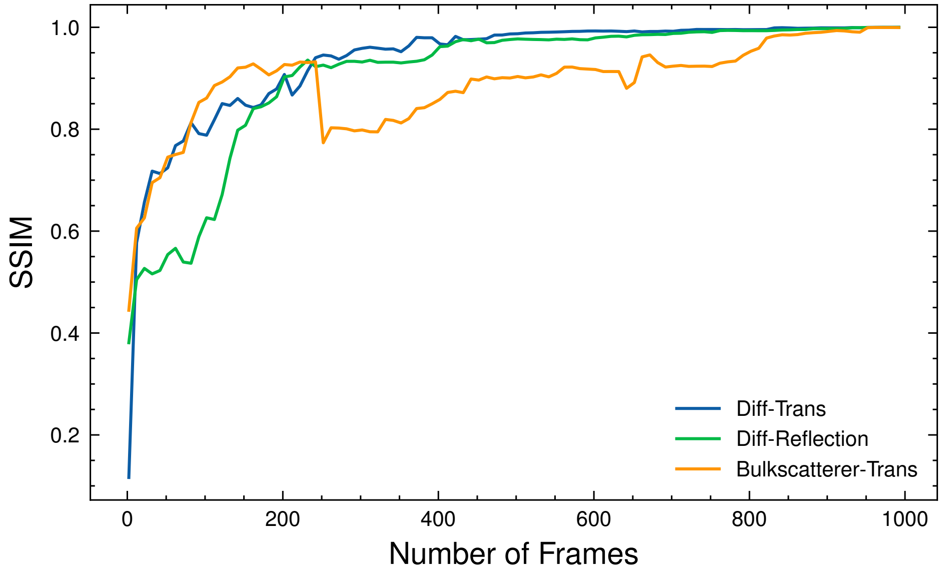


FIG. S2. SSIM as a function of the number of frames used for object reconstruction, compared to the ground truth with 1000 frames.

$$E_i(t) = |E_0| e^{j(\omega_i t + \varphi_i)}, \tag{S17}$$

where $|E_0|$ denotes the amplitude of the electric field, $\omega_i$ is the frequency of the field, and $\varphi_i$ is the phase. If the interferometer is not balanced in electric field amplitude, this can introduce additional complexity to our analysis.

To measure the intensity at each output port, we define the intensities in terms of the electric fields:

$$I_i(t_1, t_2) = \langle E_i^*(t_1, t_2, t) E_i(t_1, t_2, t) \rangle, \tag{S18}$$

where $\langle \cdot \rangle$ represents the ensemble average over $t$. The intensity at port A can be computed with S16 as follows:

$$I_A(t_1, t_2) = \frac{|E_0|^2}{2} \langle \left[ e^{j(\omega_1(t-t_1)+\varphi_1)} + j e^{j(\omega_2(t-t_2)+\varphi_2)} \right] \left[ e^{-j(\omega_1(t-t_1)+\varphi_1)} - j e^{-j(\omega_2(t-t_2)+\varphi_2)} \right] \rangle. \tag{S19}$$

Next, we consider the finite coherence length by accounting for the non-zero spectral bandwidth, which necessitates adding a mutual coherence term $g^{(1)}_{(t_2-t_1)}$ that describes the degree of coherence between the two electric fields [S5]. We can then rewrite the intensity at port A as:

$$I_A(t_1, t_2) = \frac{|E_0|^2}{2} \langle 2 + |g^{(1)}_{(t_2-t_1)}| \left( j e^{j(\omega_2(t-t_2)+\varphi_2)} e^{-j(\omega_1(t-t_1)+\varphi_1)} - j e^{j(\omega_1(t-t_1)+\varphi_1)} e^{-j(\omega_2(t-t_2)+\varphi_2)} \right) \rangle. \tag{S20}$$

To simplify this further, we can apply the trigonometric identity $\sin(x) = \frac{e^{jx} - e^{-jx}}{2j}$. The intensity at port A can now be expressed as:

$$I_A(t_1, t_2) = |E_0|^2 \left( 1 + |g^{(1)}_{(t_2-t_1)}| \langle \sin(\omega_2 t_2 - \omega_1 t_1 - \Delta\omega t - \Delta\varphi) \rangle \right), \tag{S21}$$

where $\Delta\omega = \omega_2 - \omega_1$ is the frequency difference of the fields in both paths, and $\Delta\varphi = \varphi_2 - \varphi_1$ is the phase difference. In the case where the frequencies are identical ($\omega_1 = \omega_2 = \omega$) and assuming coherent inputs, where the phase difference $\Delta\varphi$ remains constant, we can simplify the expression by substituting $\Delta t = t_2 - t_1$:

$$I_A(\Delta t) = |E_0|^2 \left( 1 + |g^{(1)}_{(\Delta t)}| \sin(\omega \Delta t - \Delta\varphi) \right). \tag{S22}$$

The intensity at port B can be written correspondingly as:

$$I_B(\Delta t) = |E_0|^2 \left( 1 - |g^{(1)}_{(\Delta t)}| \sin(\omega \Delta t - \Delta\varphi) \right). \tag{S23}$$

In the case of mutually incoherent fields $E_1$ & $E_2$, where the phase difference $\Delta\varphi$ varies randomly during a measurement, the sinusoidal term averages out to zero, resulting in no measurable interference. In this scenario, the intensities at both ports become equal:

$$\begin{aligned} I_A(\Delta t) &= |E_0|^2 = I_0, \\ I_B(\Delta t) &= |E_0|^2 = I_0. \end{aligned} \tag{S24}$$

Moving on to second-order correlations, the second-order correlation function is defined as [S6, S7]:

$$g^{(2)}(t_1, t_2) = \frac{\langle E_1^*(t_1) E_2^*(t_2) E_1(t_2) E_2(t_1)\rangle}{\langle |E_1(t_1)|^2\rangle\langle |E_2(t_2)|^2\rangle}. \tag{S25}$$

By expressing the second-order correlation function in terms of classical intensities, we can rewrite it as:

$$g^{(2)}(t_1, t_2) = \frac{\langle I_1(t_1) I_2(t_2)\rangle}{\langle I_1(t_1)\rangle\langle I_2(t_2)\rangle}. \tag{S26}$$

To simplify the notation, we can redefine the time variables such that $t_1 = t$ and $t_2 = t + \tau$. Furthermore we add a new variable $\Delta t$ which defines the optical delay between the two arms of the interferometer. Hence, substitute $I_i$ for $I_X(t, \Delta t)$ or $I_Y(t, \Delta t)$:

$$g^{(2)}_{XY}(\Delta t, \tau) = \frac{\langle I_X(t, \Delta t) I_Y(t + \tau, \Delta t)\rangle}{\langle I_X(t, \Delta t)\rangle\langle I_Y(t, \Delta t)\rangle}. \tag{S27}$$

In this context, there are three important time variables to consider:

- **t**: The global time, representing the overall temporal evolution of the system. Variations with respect to this time can typically be averaged out across the ensemble, as they tend to be much faster than the exposure time.
- $\Delta t$: The interferometric delay, which is a key parameter in ToF measurements and is the primary variable of interest when determining optical path differences.
- $\tau$: The relative time delay between two intensity measurements in the $g^{(2)}$. This parameter is crucial for analysing the decorrelation time, helping us assess how long the intensities remain correlated before decoherence effects take over.

Initially, the primary focus is on the degree of correlation for a specific interferometer delay. We can simplify our analysis by assuming we have the ideal case where the system immediately decorrelates to a value of 1 [S8].

Therefore, we only need to examine the correlation at the point where $\tau = 0$, allowing us to measure the maximum correlation directly without the need to evaluate the entire decorrelation curve.

There are two approaches to measuring second-order correlations in an interferometer. One can either measure the auto-correlation of the intensity at a single port or the cross-correlation between the intensities at two different ports. For cross-correlation, using the intensities from both ports A and B, and assuming $\langle I_i(t_i)\rangle = I_0$, we obtain:

$$g^{(2)}_x(\Delta t) = \frac{I_0^2\langle 1 - |g^{(1)}_{(\Delta t)}|^2 \sin^2(\omega\Delta t - \Delta\varphi)\rangle}{I_0^2}. \tag{S28}$$

For the auto-correlation, using the intensity at only one port, the second-order correlation function becomes:

$$g^{(2)}_a(\Delta t) = \frac{I_0^2\langle 1 + 2|g^{(1)}_{(\Delta t)}| \sin(\omega\Delta t - \Delta\varphi) + |g^{(1)}_{(\Delta t)}|^2 \sin^2(\omega\Delta t - \Delta\varphi)\rangle}{I_0^2} \tag{S29}$$

With a completely stable phase between the two arms, oscillatory terms appear in the $g^{(2)}$. However, for a varying phase over time $t$ across the entire angular range $(0, 2\pi)$, the expectation values of the terms simplify as $\langle\sin(x)\rangle = 0$ and $\langle\sin^2(x)\rangle = 0.5$. This gives the final expressions:

$$\begin{aligned} g^{(2)}_x(\Delta t) &= 1 - \frac{|g^{(1)}_{(\Delta t)}|^2}{2}, \\ g^{(2)}_a(\Delta t) &= 1 + \frac{|g^{(1)}_{(\Delta t)}|^2}{2}. \end{aligned} \tag{S30}$$

This result indicates that we observe a smooth dip (anti-bunching) or peak (bunching) in the $g^{(2)}$ correlation function. When the two paths have zero delay ($\Delta t = 0$), the correlation is maximal, and as the delay increases, the correlation decreases, following a Gaussian profile, eventually approaching 1, depending on the mutual coherence length of the two fields. The maximum visibility of 50 arises from the use of classical fields; in a quantum framework, this visibility can be significantly higher [S9]. The degree of visibility is directly dependent on the first-order coherence, $g^{(1)}_{(\Delta t)}$, which varies from 0 for incoherent fields to 1 for fully coherent fields. In this specific case of equal intensities in both arms the visibility of the resulting interference pattern is related to the absolute value of the first-order coherence $|g^{(1)}|$.

Up to this point, we have discussed the scenario where a field with a single wavelength band of non-zero bandwidth field enters the interferometer and is split into two, resulting in matched frequencies in both arms of the interferometer. Now, we extend this analysis to the case where two distinct fields, each with a different frequency, enter the interferometer. This situation leads to multiple frequencies propagating through both arms, resulting in more complex interference dynamics. Instead of dealing with just two fields, we now have four fields inside the interferometer, two associated with each input.

Continuing with the same argumentation from the previous section, at the output ports $A$ and $B$, the electric fields can be described as follows:

$$\begin{aligned} E_A(t_1, t_2, t) &= \frac{1}{\sqrt{4}} \left[ E_{\omega_1}(t - t_1) + jE_{\omega_2}(t - t_2) + E_{\omega_3}(t - t_1) + jE_{\omega_4}(t - t_2) \right], \\ E_B(t_1, t_2, t) &= \frac{1}{\sqrt{4}} \left[ E_{\omega_2}(t - t_2) + jE_{\omega_1}(t - t_1) + E_{\omega_4}(t - t_2) + jE_{\omega_3}(t - t_1) \right], \end{aligned} \tag{S31}$$

Here, each $E_{\omega_i}(t)$ represents the electric field associated with a specific frequency $\omega_i$. These fields correspond to the different input frequencies after passing through the interferometer. The two paths ($t_1$ and $t_2$) represent the travel times through the respective arms.

In this scenario, two approaches exist for computing the second-order correlation function $g^{(2)}$, that will depend on the experimental configuration and wavelength separation of the two bands.

**Measurement through Bandpass Filtering:** One approach focuses on measuring the second-order correlation by filtering the frequencies $\omega_1$ at port A and $\omega_2$ at port B. This method allows for the direct assessment of the correlation between the two input fields at separate output ports. By isolating these specific frequencies, we can gain insights into their individual contributions to the overall correlation.

**Cross-Detection of Input Fields:** Alternatively, we can detect both $\omega_1$ and $\omega_2$ at both ports A and B. This setup enables us to explore cross terms between the two input fields, by calculating the $g^{(2)}$ from a single port. Such an approach offers a more integrated view of the relationship between the input fields and their collective behaviour at the output.

For the case of filtering specific frequencies at each port, the intensities at the output ports $A$ and $B$ are given by the following equations using Eq. S18:

$$\begin{aligned} I_A(\Delta t) &= |E_0|^2 \left( 1 + |g^{(1)}_{(\Delta t, I)}| \sin\left(\omega_I \Delta t - \Delta\varphi\right) \right), \\ I_B(\Delta t) &= |E_0|^2 \left( 1 - |g^{(1)}_{(\Delta t, II)}| \sin\left(\omega_{II} \Delta t - \Delta\varphi\right) \right), \end{aligned} \tag{S32}$$

where $\omega_I$ and $\omega_{II}$ are the respective frequencies of the input fields, and $g^{(1)}$ represents the first-order coherence function.

Using the intensity correlation function Eq. S26 to calculate the second-order auto-correlation for one port, we obtain:

$$g^{(2)}_{AA/BB}(\Delta t) = 1 + \frac{|g^{(1)}_{(\Delta t)}|^2}{2}. \tag{S33}$$

This leads to a peak in the second-order correlation function, similar to the single-field case. However, when performing a cross-correlation between the two output ports, the second-order correlation becomes:

$$g^{(2)}_x(\Delta t) = \frac{I_0^2 \langle 1 - |g^{(1)}_{(\Delta t, I)}| \sin\left(\omega_I \Delta t - \Delta\varphi\right) |g^{(1)}_{(\Delta t, II)}| \sin\left(\omega_{II} \Delta t - \Delta\varphi\right) \rangle}{I_0^2}. \tag{S34}$$

We can further simplify this expression using the trigonometric identity $\sin(x)\sin(y) = \frac{1}{2}[\cos(x - y) - \cos(x + y)]$, yielding:

$$g_x^{(2)}(\Delta t) = \langle 1 - 0.5|g^{(1)}_{(\Delta t,I)}||g^{(1)}_{(\Delta t,II)}| \left[\cos\left(\Delta\omega\Delta t\right) - \cos\left((\omega_I + \omega_{II})\Delta t - 2\Delta\varphi\right)\right]\rangle. \tag{S35}$$

The second cosine term averages out to zero due to the ensemble averaging process, leaving:

$$g_x^{(2)}(\Delta t) = 1 - |g^{(1)}_{(\Delta t,I)}||g^{(1)}_{(\Delta t,II)}| \frac{\cos\left(\Delta\omega\Delta t\right)}{2}. \tag{S36}$$

Thus, we observe an oscillating term that arises when cross-correlating the two filtered output fields of the interferometer with different input frequencies. However, in the auto-correlation scenario, we still recover the same result as for the single input field case.

In this configuration, all input fields are present at both output ports, allowing for a comprehensive analysis of their interactions. The intensities at each port, derived from Eq. S18, are expressed as follows:

$$\begin{aligned} I_A &= \frac{I_0}{2}\left[2 - \sin\left(\omega_I\Delta t + \Delta\varphi\right) - \sin\left(\omega_{II}\Delta t + \Delta\varphi\right)\right], \\ I_B &= \frac{I_0}{2}\left[2 + \sin\left(\omega_I\Delta t + \Delta\varphi\right) + \sin\left(\omega_{II}\Delta t + \Delta\varphi\right)\right]. \end{aligned} \tag{S37}$$

By substituting these intensity expressions into the second-order correlation function defined in Eq. S26, we obtain the correlation functions for the same port measurements:

$$g_a^{(2)} = I_0^2\left[1 + \frac{1}{8}|g^{(1)}_{(\Delta t,I)}|^2 + \frac{1}{8}|g^{(1)}_{(\Delta t,II)}|^2 + \frac{1}{4}|g^{(1)}_{(\Delta t,I)}||g^{(1)}_{(\Delta t,II)}|\cos(\Delta\omega\Delta t)\right]. \tag{S38}$$

When cross-correlating the outputs from both ports, the correlation function takes the form:

$$g_x^{(2)} = I_0^2\left[1 - \frac{1}{8}|g^{(1)}_{(\Delta t,I)}|^2 - \frac{1}{8}|g^{(1)}_{(\Delta t,II)}|^2 - \frac{1}{4}|g^{(1)}_{(\Delta t,I)}||g^{(1)}_{(\Delta t,II)}|\cos(\Delta\omega\Delta t)\right]. \tag{S39}$$

In this scenario, the sinusoidal term also emerges, introducing an oscillatory behaviour in the correlation function. However, it is important to note that the visibility of this correlation is reduced compared to the filtered case. This reduction in visibility reflects the more complex interactions occurring when both input fields are detected simultaneously, as opposed to when individual fields are isolated at the output.


[S1] Joseph W Goodman. *Introduction to Fourier optics*. Roberts and Company publishers, 2005.
[S2] Kedar Khare, Mansi Butola, and Sunaina Rajora. *Fourier optics and computational imaging*. Springer, 2015.
[S3] Miguel A. Quetzeri-Santiago, Alfonso A. Castrejón-Pita, and J. Rafael Castrejón-Pita. The Effect of Surface Roughness on the Contact Line and Splashing Dynamics of Impacting Droplets. *Scientific Reports*, 9(1), 12 2019.
[S4] Florian Willomitzer, Prasanna V Rangarajan, Fengqiang Li, Muralidhar M Balaji, Marc P Christensen, and Oliver Cossairt. Supplementary material to: Fast non-line-of-sight imaging with high-resolution and wide field of view using synthetic wavelength holography. *Nature Communications*, 12(1):1–11, 2021.
[S5] Grant R Fowles. *Introduction to modern optics*. Courier Corporation, 1989.
[S6] Roy J Glauber. The quantum theory of optical coherence. *Physical Review*, 130(6):2529, 1963.
[S7] Marlan O Scully and M Suhail Zubairy. *Quantum optics*. Cambridge university press, 1997.
[S8] Joseph W Goodman. *Speckle phenomena in optics: theory and applications*. Roberts and Company Publishers, 2007.
[S9] Rodney Loudon. *The quantum theory of light*. OUP Oxford, 2000.
